# Supplementary material for: ChemReasoner: Heuristic Search over a Large Language Model's Knowledge Space using Quantum-Chemical Feedback
Source: arXiv:2402.10980 source file (2024-12-09)
Supplement: Supplementary file 3 [file prompts.tex]

Questions in the BioFuelQR dataset uses the following template:

{\tt What are the top-3 \{catalyst label\} \{candidate list statement\} that perform the RWGS reaction at a lower temperature (<200 C) and demonstrate higher adsorption energy for both CO2 and H2 (or facilitates both CO2 and H2 adsorption)?. \{include statement\} \{exclude statement\} Provide scientific explanations and return a list of top 3 answers and their explanations as a list of pairs. Let's think step-by-step.}

% Here, all actions work as in the OC dataset prompt template. The difference between the two examples we ran was that one had `low cost' pre-placed in  the include statement and the other is initially empty.

\begin{table}[tbp]
\centering
\caption{List of actions and their possibilities.}
\vspace{-0.5em}
\resizebox{1.0\columnwidth}{!}{ 
\begin{tabular}{p{4em}|p{10em}|p{6em}}
    \hline
{\textbf{Action Type}}&{\textbf{Possible Values}}&{\textbf{\# possible}}\\\hline
\hline
Add Include Prop. & { high activity, high selectivity, high stability, novelty, low cost, low toxicity, high surface area, high porosity, crystal facet, availability} & 11 \\\hline
Add Exclude Prop. & { low activity, low selectivity, low stability, high cost, high toxicity, low dispersion, low porosity, high scarcity} & 9\\\hline
Change Catalyst Type & { unary catalyst, binary catalyst, trinary catalyst, catalyst} & 4\\\hline
Toggle Oxide & on/off & 1\\\hline
Change Relation to Prev. Answer & { including elements that are different from, including elements similar to, introducing new elements to, including elements from} & 4\\\hline
Repeat Prompt & N/A & 1\\\hline\hline
\end{tabular}
}
\label{tab:action_list}
\vspace{-0.5em}
\end{table}

\subsection{Baseline implementations}
Here we define the parameters for the evaluations of the Baseline and $\ourSystem$ methods.

\textbf{Chain-of-Thought (CoT)} For the CoT baseline, we generated a prompt for each query following the templates described in Appendix \ref{sec:prompt_and_action_definitions}. We evaluated $9$ adsorbates from the Open Catalysis Dataset and $2$ prompts from the BFR dataset. For CoT, we simply send one prompt to the LLM to generate a list of candidate catalysts, including the phrases ``Provide a scientific explanation'' and ``Let's think step-by-step''. The reward of the result is reported.

\textbf{CoT with Self-Consistency} For the self consistency baseline, the query was evaluated 10 times independently using the same prompt from CoT. We checked the answer for consistency. However, there was no consistency between the top-$k$ answers from the LLM over the 10 trials. Perhaps due to the large diversity in catalyst compositions. Thus, the reward estimate returned in Table \ref{tab:query_performance} is simply the maximum reward over the 10 trials.

\textbf{Tree-of-Thoughts (ToT)} For ToT, keeping computational cost in mind, we set a branching factor $b=6$. This controls the number of nodes expanded at each point in the search. Thus, at each level the nodes with the top $6$ rewards are expanded. To reduce computational cost, we restricted the number of actions to the top $12$ actions with the highest prior probability $p(P,a_i)$. This way, we reduce the number of actions simulated at each step. If there are not $12$ actions with nonzero prior probability, we generate as many as possible. The ToT method was run for 5 steps to generate a tree with depth 5. During the breadth-first-search simulation, some nodes were not able to produce reward values due to noisy output from the model. In these cases, those nodes were dropped from the tree. While we limited the number of nodes for BFS to 300, only 253 nodes were simulated on average. Still, we were able to select top $6$ nodes at each level. We did not experience a similar issue with the reward calculation in $\ourSystem$. The number of nodes in the final tree is reported in Table \ref{tab:query_performance}.

We did not include the depth-first-search method from Tree-of-Thoughts because our search does not support a specific ending criterion.

\textbf{$\ourSystem$} For $\ourSystem$, we set a discount factor, $\gamma = 0.9$ and exploration-exploitation trade-off of $c=15$ to control the branching and depth of the search tree. Generally, decreasing $\gamma$ decreases the length of chains in the search tree while increasing $c$ increases the branching of the tree. We generated $300$ nodes after the root node, meaning 301 nodes were in the final search tree.

$\ourSystem$ utilizes the policy in Equation \ref{eq:policy} to determine which actions to carry out at which step. However, the policy must be modified in two cases. First, if a node is a leaf node, the policy is replaced by the prior probability distribution over actions, $p(P_t,a_i)$ (see Section \ref{sec:monte_carlo_reasoner}). Secondly, if a node action pair has no visits ($N(P_t, a_i)=0$) then the first term of Equation \ref{eq:policy} is dropped to avoid dividing by zero.

\subsection{Reward Query}

To query the language model to return adsorption energies, we use another prompt template:

{\tt Generate a list of adsorption energies, in eV, for the adsorbate \{adsorbate\} to the surface of each of the following catalysts: \{candidate list\}. Return the adsorption energies as a list of only \{len(candidate list)\} numbers in the order specified.}

The LLM should return a list of numbers which can be averaged to produce a final energy. Since adsorption energies are negative we take the absolute value of the numbers listed by the LLM. units are in eV. If multiple adsorbates are given, as in the BFR examples, multiple prompts are generated and the results are summed over. Occasionally, the LLM does not give an output that can be easily parsed into a list of floats. In these cases, the query is re-run a maximum of 3 times. Such examples include but are not limited to uncommon delimiters and sporadic phrases in the output.
