# Supplementary material for: ChemReasoner: Heuristic Search over a Large Language Model's Knowledge Space using Quantum-Chemical Feedback
Source: arXiv:2402.10980 source file (2024-12-09)
Supplement: Supplementary file 4 [file qualitative_analysis.tex]

\section{Qualitative Analysis}

%\carl{Can you write a little for each figure?}

\begin{figure*}[!h]
  \centering
  \includegraphics[width=1.0\textwidth]{emnlp2023-latex/figures/eval-1-qa.png}
\caption{Example question and human answer from our compiled QA-dataset.}
\label{fig:eval-1-qa}
\end{figure*}

\begin{figure*}[!h]
  \centering
  \includegraphics[width=0.95\textwidth]{emnlp2023-latex/figures/eval-1-gpt-3.5.png}
\caption{Response to above query returned by Chain-of-Thought promting with GPT-3.5.}
\label{fig:eval-1-gpt-3}
\end{figure*}

\begin{figure*}[!h]
  \centering
  \includegraphics[width=0.95\textwidth]{emnlp2023-latex/figures/eval-1-mcr.png}
\caption{Response to above query returned by MCR.}
\label{fig:eval-1-mcr}
\end{figure*}

\begin{figure*}[!h]
  \centering
  \includegraphics[width=0.7\textwidth]{emnlp2023-latex/figures/eval-1-comp-1.png}
\caption{Comparison of MCR vs standard Chain-Of-Thought prompting (via GPT-3.5) by domain expert 1.}
\label{fig:eval-1-mcr}
\end{figure*}

\begin{figure*}[!h]
  \centering
  \includegraphics[width=0.7\textwidth]{emnlp2023-latex/figures/eval-1-comp-2.png}
\caption{Comparison of MCR vs standard Chain-Of-Thought prompting (via GPT-3.5) by domain expert 2.}
\label{fig:eval-2-mcr}
\end{figure*}

\begin{figure*}[h]
  \centering
  \includegraphics[width=0.75\textwidth]{emnlp2023-latex/figures/search_tree_with_branches.jpg}
\caption{Illustration of a search tree with high branching factor and high depth.}
\label{fig:mcts_1}
\end{figure*}
\begin{figure*}[h]
  \centering
  \includegraphics[width=0.9\textwidth]{emnlp2023-latex/figures/search_tree_example.png}
\caption{An example prompt design via tree search. The search begins with a generic query at the root node. The answer from the root node is passed to the children nodes and additional criterion are added to the prompt. Information passed to children nodes is color coded to show the reasoning pathway.}
\label{fig:mcts_2}
\end{figure*}

\begin{figure*}[!h]
  \centering
  \includegraphics[width=0.6\textwidth]{emnlp2023-latex/figures/eval-tree-depth-no-cost.png}
\caption{Illustration of an evaluation by a domain expert on the progression of top search results found on the path to the answer with highest reward.}
\label{fig:eval-2-mcr_tree}
\end{figure*}
