# Supplementary material for: ChemReasoner: Heuristic Search over a Large Language Model's Knowledge Space using Quantum-Chemical Feedback
Source: arXiv:2402.10980 source file (2024-12-09)
Supplement: Supplementary file 9 [file rewards.tex]

\section{Additional Analysis}

\subsection{Robustness of GNN Rewards}
Does ChemReasoner's performance improve using higher number of iterations for relaxation?

\subsection{How robust are different reward functions?}
Plot distribution of LLM and GNN rewards for the candidates we have DFT rewards for.
